# Supplementary material for: Combined Flux and Anisotropy Searches Improve Sensitivity to Gamma Rays from Dark Matter
Source: arXiv:1312.3945 ancillary file (2013-12-13)
Supplement: Supplementary file 1 [file Supplemental_Material.pdf]

# Supplemental Material for "Combined Flux and Anisotropy Searches Improve Sensitivity to Gamma Rays from Dark Matter"

Sheldon S. Campbell[1,2] and John F. Beacom[1,2,3]
[1]Center for Cosmology and AstroParticle Physics (CCAPP), Ohio State University, Columbus, OH 43210
[2]Department of Physics, Ohio State University, Columbus, OH 43210
[3]Department of Astronomy, Ohio State University, Columbus, OH 43210
(Dated: December 13, 2013)

This supplement provides additional details about the calculation of the line constraints that are not necessary to understand the results in the Letter, but provide further insight into the methods introduced.

At an energy of 135 GeV, we approximate the acceptance (effective area integrated over the field of view) of Fermi-LAT to be $A = \varepsilon\Omega \simeq 2 \times 10^4$ cm$^2$ sr [1], and that of GAMMA-400 to be 5/8 as large [2]. Observations of the diffuse $\gamma$-ray background (DGRB) are done in an unmasked fraction $f_{\rm sky} \simeq 0.325$ of the sky [3]. Since data from the masked region are removed, it is convenient to introduce the exposed acceptance $A_{\rm exp} \equiv Af_{\rm sky}$. Then the number flux associated with $N_\gamma$ gamma rays detected in time $t$ is

$$\Phi_{\rm tot} = \frac{N_\gamma}{A_{\rm exp}t}.$$

The contributions to the DGRB are broken into components

$$\Phi_{\rm tot} = \Phi_{\rm line} + \Phi_{\rm BG},$$

a spectral line of flux $\Phi_{\rm line}$ presumed to be dark matter annihilation, and a background flux $\Phi_{\rm BG}$ due to all other unresolved sources. The line comes from annihilations in our galaxy's halo and from extragalactic dark matter. The extragalactic line is smeared by integration over redshift, but since low redshifts are the most important, the signal is nearly a line within a reasonable energy bin (see e.g., Ref. [4]). One way to write this is

$$\Phi_{\rm line} = (B_{\rm sub} + B_{\rm eg})\Phi_{\rm sm},$$

where $\Phi_{\rm sm}$ is the flux associated with annihilations in the smooth component of our Galactic halo, and this is weighted by boost factors that parametrize our ignorance about further details of the dark matter distribution. Contributions from dark matter substructure in the halo are encoded in the boost factor $B_{\rm sub}$, and the extragalactic flux is determined from $B_{\rm eg}$. In this work, we consider a scenario where the extragalactic contribution is negligible, although there are other viable cases where the extragalactic contribution is important.

A line signal has significance $N_\sigma$ if

$$\Phi_{\rm tot} - \Phi_{\rm BG} = \Phi_{\rm line} = N_\sigma \sigma_\Phi,$$

where $\sigma_\Phi$ is the uncertainty (taken here to be statistical) of the flux measurement:

$$\sigma_\Phi \simeq \frac{\sigma_N}{A_{\rm exp}t} = \frac{\sqrt{N_\gamma}}{A_{\rm exp}t} = \sqrt{\frac{\Phi_{\rm tot}}{A_{\rm exp}t}} = \sqrt{\frac{\Phi_{\rm BG} + B_{\rm sub}\Phi_{\rm sm}}{A_{\rm exp}t}}.$$

To observe a signal of significance $N_\sigma$, the substructure boost factor must therefore satisfy

$$B_{\rm sub}\Phi_{\rm sm} = \sqrt{\frac{\Phi_{\rm BG} + B_{\rm sub}\Phi_{\rm sm}}{T_\Phi}},$$

or

$$B_{\rm sub} = \frac{1 + \sqrt{1 + 4T_\Phi \Phi_{\rm BG}}}{2T_\Phi \Phi_{\rm sm}}, \tag{1}$$

where

$$T_\Phi \equiv A_{\rm exp}\frac{t}{N_\sigma^2}.$$

The line flux from the smooth galactic halo in the unmasked sky was estimated in this example to be

$$\Phi_{\rm sm} \simeq 2.2 \times 10^{-11}\ {\rm ph\ cm^{-2}\ s^{-1}\ sr^{-1}}.$$

The DGRB flux at 135 GeV in an energy bin of width of the instrument energy resolution (10% for Fermi-LAT and 1% for GAMMA-400) was estimated to be

$$\Phi_{\rm BG} \simeq \begin{cases} 2.2 \times 10^{-10}\ {\rm ph\ cm^{-2}\ s^{-1}\ sr^{-1}} & \text{for Fermi-LAT,} \\ 2.2 \times 10^{-11}\ {\rm ph\ cm^{-2}\ s^{-1}\ sr^{-1}} & \text{for GAMMA-400.} \end{cases}$$

The numerical similarity with $\Phi_{\rm sm}$ is coincidental. In reality, one would expect the background flux for GAMMA-400 to be even lower, since its sharp angular resolution would allow it to resolve more point sources whose flux would no longer contribute to the diffuse background.

We now apply the same logic to the mean-weighted angular power spectrum line search. A line signal of significance $N_\sigma$ satisfies

$$\tilde{C} - \tilde{C}_0 = N_\sigma \sigma_{\tilde{C}}.$$

Our examples use $\tilde{C}_0 = 7 \times 10^{-6}$ sr [3]. Assuming the angular power is shot-noise-dominated and statistics limited, and $B_{\rm sub} - 1$ is above the threshold described in the main article, then the measurement uncertainty is

$$\sigma_{\tilde{C}} \simeq \frac{\tilde{C}_{\rm sub}}{\tilde{C}_{{\rm sub},\ell_1}}\frac{\kappa}{N_\gamma},$$

where

$$\kappa \equiv 8\pi\sqrt{f_{\rm sky}}\sigma_b e^{\sigma_b^2\ell_1^2},$$

$\sigma_b$ is the experiment beam width (approximated as Gaussian), and $\ell_1$ is the lower bound of the range of multipoles the angular power spectrum is averaged over. In our calculations, we used $\ell_1 = 155$, and estimated

$$\sigma_b \simeq \begin{cases} 0.0018 \text{ sr for Fermi-LAT,} \\ 0.00018 \text{ sr for GAMMA-400.} \end{cases}$$

The total angular power is broken into components as

$$\tilde{C} = \left(\frac{\Phi_{\rm tot} - \Phi_{\rm sub}}{\Phi_{\rm tot}}\right)^2 \tilde{C}_0 + \left(\frac{\Phi_{\rm sub}}{\Phi_{\rm tot}}\right)^2 \tilde{C}_{\rm sub},$$

where $\tilde{C}_{\rm sub}$ is the mean-weighted fluctuation angular power spectrum of the halo substructure, and

$$\Phi_{\rm sub} = (B_{\rm sub} - 1)\Phi_{\rm sm}$$

is the flux from substructure. Thus, we find that to observe an anisotropy line signal of significance $N_\sigma$, the halo substructure angular power must be

$$\tilde{C}_{\rm sub} = \frac{1 + \frac{F}{B_{\rm sub}-1}}{T_C \Phi_{\rm sm}(B_{\rm sub} - 1)} + \left(1 + \frac{2F}{B_{\rm sub-1}}\right)\tilde{C}_0, \qquad (2)$$

where

$$T_C \equiv \frac{\tilde{C}_{{\rm sub},\ell_1}}{\tilde{C}_{\rm sub}} \frac{A_{\rm exp} t}{\kappa N_\sigma}, \;\; F \equiv 1 + \frac{\Phi_{\rm BG}}{\Phi_{\rm sm}}.$$

Fig. 1 shows the halo substructure parameter space where signals for the 135 GeV line of at least $2\sigma$ significance are expected to be observed. Note that the vertical flux lines are determined by $t/N_\sigma^2$, while the anisotropy lines are determined by $t/N_\sigma$. We estimated $\tilde{C}_{{\rm sub},\ell_1}/\tilde{C}_{\rm sub} \approx 1.6$. The value of this ratio simply scales $t$ or $N_\sigma$.

For the 1-year data of the Fermi-LAT, the angular power of halo substructure would need to be high, $\tilde{C}_{\rm sub} \gtrsim 0.03$ sr, in order for the anisotropy data to extend the sensitivity of the flux methods to dimmer substructure. In the 5-year data, one sees that a $2\sigma$ flux signal would be not be seen in the anisotropy. This shows that a weak hint of a signal would likely be first apparent in the flux data. However, as was shown in the main article, if $B_{\rm sub} \lesssim 4$, then observation of a $5\sigma$ signal is beyond the reach of the flux data, but may be seen in the anisotropy data if $\tilde{C}_{\rm sub} \gtrsim 0.01$ sr.

In GAMMA-400, the anisotropy is important, even at $2\sigma$, after just 1 year of data. After 5 years, though, the entire substructure parameter space is probed to $2\sigma$ by the flux, which is predicted to be sensitive to the 135 GeV line in the DGRB in the complete absence of halo substructure. In the scenario described here, the anisotropy provides a substantial improvement to the significance of the signal when $\tilde{C}_{\rm sub} \gtrsim 0.001$ sr. Importantly, this would tell us much more about the substructure properties.

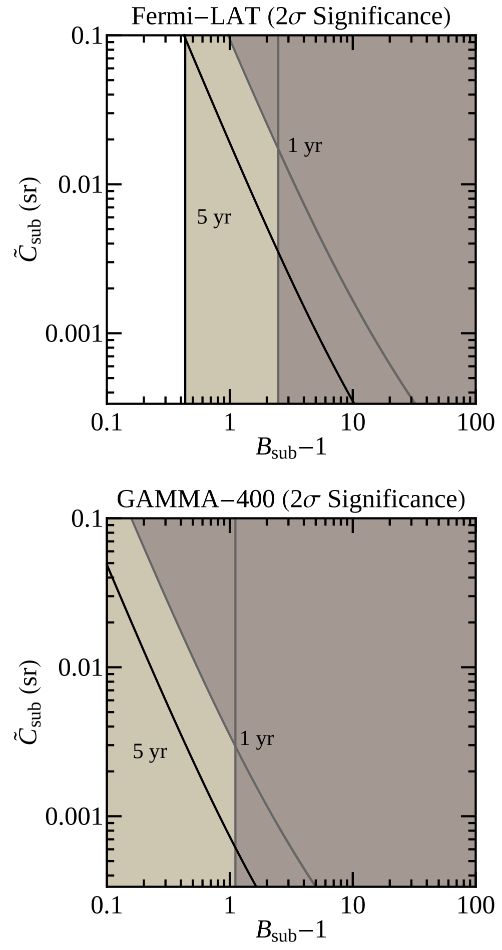


FIG. 1: The parameter space where the 135 GeV line is expected to be observed in the DGRB with a signal strength of $2\sigma$ (the $5\sigma$ sensitivity is shown in Fig. 2 of the main article). The vertical lines are flux constraints of Eqn. (1), while the diagonal curves are the anisotropy constraints given by Eqn. (2). The soft lines show the reach after 1 year of data, and the solid lines show 5 years.

[1] P7_V6 acceptance, http://www.slac.stanford.edu/exp/glast/groups/canda/archive/pass7v6/lat_Performance.htm

[2] A. M. Galper, O. Adriani, R. L. Aptekar, I. V. Arkhangelskaja, A. I. Arkhangelskiy, G. A. Avanesov, L. Bergstrom and E. A. Bogomolov *et al.*, arXiv:1306.6175 [astro-ph.IM].

[3] M. Ackermann *et al.* [Fermi LAT Collaboration], Phys. Rev. D **85**, 083007 (2012) [arXiv:1202.2856 [astro-ph.HE]].

[4] J. F. Beacom, N. F. Bell and G. D. Mack, Phys. Rev. Lett. **99**, 231301 (2007) [astro-ph/0608090].
